# Supplementary material for: Tetrahedral Elliptic Curves and the local-global principle for Isogenies
Source: arXiv:1306.6818 ancillary file (2014-05-02)
Supplement: Supplementary file 1 [file X13.pdf]

# Computing the modular curves $X_{\text{sp}}(13)$ , $X_{\text{ns}}(13)$ and $X_{A_4}(13)$ using modular symbols in Sage

J. E. Cremona, B. S. Banwait

August 16, 2013

## Abstract

This document is an annotated version of a Sage script which computes the three genus 3 modular curves  $X_{\text{sp}}(13)$ ,  $X_{\text{ns}}(13)$  and  $X_{A_4}(13)$  of level 13.

## 1 Preliminaries: defining the congruence subgroup and modular symbol space

We set the level and define the congruence subgroup  $G = \tilde{\Gamma}(13) = \Gamma_0(13^2) \cap \Gamma_1(13)$ , which is conjugate to  $\Gamma(13)$ :

```
N = 13
G = GammaH(N^2, [N+1])
```

Next we define the associated modular symbol space  $MG$  (with sign 0), and its cuspidal subspace  $C$ .

```
M = ModularSymbols(G, sign=0)
C = M.cuspidal_subspace()
d = C.dimension()
```

The dimension of  $C$  is  $d = 100$  which is twice the genus of the associated modular curve  $\tilde{X}(13)$ . For future reference we will need the basis for  $C$  in terms of the ambient modular symbols space  $M$  which has dimension 183, and the matrix defining  $C$  as a subspace of  $M$ .

```
Cb = C.basis()
Cmat = Matrix([c.list() for c in Cb]).transpose()
```

Next we decompose the cuspidal space into old and new subspaces, then decompose the new part into simple components with respect to the Hecke action:

```
Cold = C.old_subspace()
Cnew = C.new_subspace()
Cnew_dec = Cnew.decomposition()
```

The number of simple new summands is 10 and their dimensions are

```
sage: [c.dimension() for c in Cnew_dec]
      [4, 4, 4, 6, 6, 8, 12, 12, 12, 24]
```

Important remark on row and column vectors and matrices: I think of elements of the modular symbol space (specifically  $C$ ) as represented by column vectors (of length 100 for  $C$ ), and so the matrices which represent operators act by multiplying these vectors on the left. We construct  $T$  and  $\text{Conj}$  like this below. However, Sage’s default is that matrices act by right multiplication of row vectors. So when we compute  $W_{13}$  using Sage’s `atkin_lehner` function we have to transpose it to be compatible with the  $T$  we compute “manually”. Later, we form various subspaces of  $\mathbb{Q}^{100}$  (and  $F^{100}$  for various fields  $F$ ), which are always given by a basis matrix of size  $d \times 100$  (where  $d$  is the dimension of the subspace) whose rows are an echelon basis.

Also, Sage makes no distinction between row and column vectors.

## 2 Computation of Hecke and other operators to get the representation of $\text{PSL}(2, 13)$ on the modular symbol space

Computation of  $\tilde{T} = \begin{pmatrix} 1 & 1/13 \\ 0 & 1 \end{pmatrix}$ : the images of the generating symbols are:

```
T_ims = [ C(sum([ s[0] * sum([ mm[0]*mm[1].manin_symbol_rep()
                        for mm in s[1].apply([1,1/N,0,1])])
                for s in c.modular_symbol_rep()))
          for c in Cb]
```

We use these to construct the matrix:

```
T = Matrix([(Cmat\vector(im.list())).list() for im in T_ims]).transpose()
```

and check it does what it should:

```
sage: all([T_ims[j] == sum([T[i,j]*Cb[i] for i in range(d)]) for j in range(d)])
      True
```

Next we compute the matrix of complex conjugation:

```
Conj = C.star_involution().matrix().transpose()
```

Next we compute the matrix of  $\tilde{S} = \begin{pmatrix} 0 & -1 \\ 121 & 0 \end{pmatrix}$ , the Atkin-Lehner involution. Note that the built-in operators (including  $T_2$  below) need to be transposed before they act on the left on column-vectors, since they are designed to act on

the right on row-vectors. From now on we will use the notation  $S, T$  instead of  $\tilde{S}, \tilde{T}$ . The Sage identifiers  $S, T$  refer to the  $100 \times 100$  matrices giving the action of these on  $C$ , identified with  $\mathbb{Q}^{100}$ .

```
W13 = C.atkin_lehner_operator()
S = W13.matrix().transpose()
```

Again we check that the action is as expected:

```
sage: all([W13(Cb[j]) == sum([S[i,j]*Cb[i] for i in range(d)]) for j in range(d)])
True
```

As a consistency check we check that that all these  $100 \times 100$  matrices have the right properties: they are the images of the standard generators of  $\mathrm{PSL}(2, \mathbb{Z})$  under the 100-dimensional representation on the cuspidal modular symbol space, which factors through  $\mathrm{PSL}(2, 13)$ .

```
sage: I = S.parent()(1)
sage: S^2 == T^N == (T*S)^3 == Conj^2 == I
True
```

Note that conjugating with  $\mathrm{Conj}$  inverts  $T$  and fixes  $S$ .

```
sage: Conj*T*Conj*T==I and Conj*S*Conj==S
True
```

We are interested in the subspace fixed by a subgroup of  $\mathrm{PSL}(2, 13)$  isomorphic to  $A_4$ . Such a subgroup is defined by taking two generating matrices in  $\mathrm{PSL}(2, 13)$ ; we choose one such subgroup (among possible conjugates) to contains  $S = \begin{pmatrix} -1 & 0 \\ 0 & 1 \end{pmatrix}$  so the corresponding congruence subgroup will be of real type. We lift the generators to  $\mathrm{PSL}(2, \mathbb{Z})$ , express them as words in the usual generators  $S, T$  of  $\mathrm{PSL}(2, \mathbb{Z})$ , and then take the same words in our  $100 \times 100$  matrices  $S, T$ .

The first generator  $A$  is  $\begin{pmatrix} -5 & 0 \\ 0 & 5 \end{pmatrix} \in \mathrm{PSL}(2, 13)$  which lifts to the element  $T^5 S T^{-2} S T^2 S T^3 S T^{-5} = \begin{pmatrix} -70 & 377 \\ -13 & 70 \end{pmatrix}$  of order 2 in  $\mathrm{PSL}(2, \mathbb{Z})$ .

```
A = T^5*S*T^(-2)*S*T^2*S*T^3*S*T^(-5)
```

The second generator  $B$  is  $\begin{pmatrix} -2 & -2 \\ -3 & 3 \end{pmatrix} \in \mathrm{PSL}(2, 13)$  which lifts to the element  $T^4 S T^3 S T^{-3} S = \begin{pmatrix} -37 & -11 \\ -10 & -3 \end{pmatrix}$  of order 3 in  $\mathrm{PSL}(2, \mathbb{Z})$ .

```
B = T^4*S*T^3*S*T^(-3)*S
```

We now verify that the group  $A_4$  generated by  $A$  and  $B$  is normalised by conjugation, and that various other identities hold. Here  $\text{Ad} = A' = B^{-1}AB \equiv \begin{pmatrix} 0 & 1 \\ 1 & 0 \end{pmatrix} \pmod{13}$ , so that  $A, A'$  commute and generate the Klein 4-subgroup of  $A_4$  whose third element is  $AA' = A'A = \begin{pmatrix} 0 & 1 \\ -1 & 0 \end{pmatrix} = S$ .

```
sage: Ad = B^(-1)*A*B
```

```
sage: Conj*A*Conj==A and Conj*B*Conj == A*B*A and A*Ad==Ad*A and A*Ad==S
```

True

To obtain the  $A_4$ -invariant subspace we construct the associated idempotent (scaled by the group order 12). Now the subspace of  $A_4$ -invariant vectors is spanned by the columns of  $\text{sigma}$ .

```
sage: sigma = (I+A)*(I+Ad)*(I+B+B^2)
```

```
sage: sigma.rank() == 6 and (sigma-12).rank() == d-6 and sigma*(sigma-12)==0
```

True

```
sage: A4_inv = sigma.column_space()
```

```
sage: A4_inv_bas = A4_inv.basis_matrix().transpose()
```

The (doubled) dimension of this  $A_4$ -invariant subspace is 6. We wish to know which of the old and new simple components this intersects. To do this we project onto each of them using the dual basis. First, the old space contains nothing  $A_4$ -invariant:

```
sage: oldproj = Cold.dual_free_module().basis_matrix()*Cmat
```

```
sage: oldproj*A4_inv_bas == 0
```

True

Next we see that two of the new components will be involved:

```
sage: newproj = [comp.dual_free_module().basis_matrix()*Cmat for comp in Cnew_dec]
```

```
sage: new_A4_components = [i for i,v in enumerate(newproj) if v*A4_inv_bas != 0]
```

```
sage: new_A4_components
```

[3, 8]

In order to compute the equation of the modular curve we could work exclusively with the sum of these two new components, which will be denoted **S3** and **S8** below. The first of these has trivial character and Hecke eigenvalues in the cubic field  $\mathbb{Q}(\zeta_7^+)$ , while the second is the sum of its twists by the order 3 character modulo 13 (denoted **chi** later). These two twists are combined here as the decomposition has been carried out over  $\mathbb{Q}$ . But it will be more convenient (specifically when computing the coordinates of the seven cusps) to work in a larger space which is  $\mathrm{PSL}(2, \mathbb{Z})$ -invariant: this is the sum of all the twists of **S3** under all the characters modulo 13, which form a cyclic group of order 12 with generator denoted **eps**.

```
S3=Cnew_dec [3]
S8=Cnew_dec [8]
comps = [3,4,6,7,8,9]
```

These components have (doubled) dimensions [6, 6, 12, 12, 12, 24].

Identifying the cupidal modular symbol space **C** with  $\mathbb{Q}^{100}$ , we denote by **V3** the subspace of  $\mathbb{Q}^{100}$  corresponding to **S3**, and by **W** the  $\mathrm{PSL}(2, \mathbb{Z})$ -invariant sum:

```
Q100 = QQ^100
V3 = Q100.subspace([C.free_module().coordinates(v)
                    for v in S3.free_module().basis()])
W = Q100.subspace(sum([[C.free_module().coordinates(v)
                       for v in Cnew_dec[c].free_module().basis()]]
                      for c in comps], []))
```

These have (doubled) dimensions 6 and 72 respectively. Note that these subspaces of  $\mathbb{Q}^{100}$  are “row subspaces”, spanned by the rows of their basis matrices, while our  $100 \times 100$  matrices **S**, **T**, **A0**, **B0**, **Conj** act on the left on column vectors. This explains the transposing which goes on in what follows.

We cut down to the +1-eigenspaces for complex conjugation (using the transpose of **Conj** for the reason just given):

```
V3plus = (Conj-1).transpose().kernel_on(V3)
Wplus = (Conj-1).transpose().kernel_on(W)
```

These have half the dimensions of **V3** and **W**, namely 3 and 36.

We compute the Hecke operator  $T_2$  (which is already transposed) and its restrictions to the two subspaces:

```
T2 = C.hecke_matrix(2)
T2V3plus = T2.restrict(V3plus)
T2Wplus = T2.restrict(Wplus)
```

### 3 Definition of various number fields

Now we define various cyclotomic fields, all contained in  $\mathbb{Q}(\zeta_{1092})$  (note that  $1092 = 2^2 \cdot 3 \cdot 7 \cdot 13$ ), with embeddings between them and some automorphisms:

```

Q1092.<zeta1092> = CyclotomicField(1092)
conj1092 = Q1092.hom([zeta1092^(-1)]) # complex conjugation on Q1092

Q13.<zeta13> = CyclotomicField(13, embedding=zeta1092^84)
eQ13Q1092 = Q13.hom([Q1092(zeta13)]) # embedding Q13 into Q1092
Q13sigma = Q13.hom([zeta13^4]) # auto of order 3 of Q13
Q13aut = Q13.hom([zeta13^2]) # auto of order 6 of Q13

Q91.<zeta91> = CyclotomicField(91, embedding=zeta1092^12)
eQ91Q1092 = Q91.hom([zeta1092^12]) # embedding Q91 into Q1092
eQ13Q91 = Q13.hom([zeta91^7]) # embedding Q13 into Q91
Q91aut = Q91.hom([zeta91^53]) # auto of order 3 of Q91 fixing Q13

Q84.<zeta84> = CyclotomicField(84, embedding=zeta1092^13)
conj84 = Q84.hom([zeta84^(-1)]) # complex conjugation on Q84
Q12.<zeta12> = CyclotomicField(12, embedding=zeta84^7)
Q7.<zeta7> = CyclotomicField(7, embedding=zeta84^12)

```

Inside  $\mathbb{Q}(\zeta_7)$  we define the cubic real subfield  $\mathbb{Q}(\zeta_7^+)$ , and inside  $\mathbb{Q}(\zeta_{13})$  the cubic subfield  $\mathbb{Q}(\zeta_{13}^{++})$  and the quartic subfield  $\mathbb{Q}(\zeta_{13}^c)$ :

```

zeta7p=zeta7+1/zeta7
Q7p.<zeta7p>=NumberField(zeta7p.minpoly(), embedding=zeta7+1/zeta7)

zeta13pp = zeta13+zeta13^5+zeta13^8+zeta13^12 # generates cubic subfield
Q13pp.<zeta13pp> = NumberField(zeta13pp.minpoly(), embedding=zeta13pp)
eQ13ppQ13 = Q13pp.hom([Q13(zeta13pp)])

zeta13c = zeta13+zeta13^3+zeta13^9 # generates quartic subfield
Q13c.<zeta13c> = NumberField(zeta13c.minpoly(), embedding=zeta13c)
eQ13cQ13 = Q13c.hom([Q13(zeta13c)])

```

For computations with  $q$ -expansions we define some power series rings:

```

ps_prec = 200
Q1092q.<q> = PowerSeriesRing(Q1092,ps_prec)
Q91q.<q> = PowerSeriesRing(Q91,ps_prec)
Q13q.<q> = PowerSeriesRing(Q13,ps_prec)
QQq.<q> = PowerSeriesRing(QQ,ps_prec)
Q13ppq.<q> = PowerSeriesRing(Q13pp,ps_prec)

```

## 4 Hecke eigenvalues and eigenvectors, and twisting operators

Now we start to compute Hecke eigenvalues (of  $T_2$ ) and associated eigenvectors. The eigenvalues of  $T_2$  on  $V_3$  are in  $\mathbb{Q}(\zeta_7^+)$  (this will be verified later). We define the first of these  $a$ , then find its three Galois conjugates, and reorder them to make sure that  $a$  is first in the list. The list of 3 conjugate eigenvalues is called `eig3`:

```
a=1/zeta7p
eig3 = a.galois_conjugates(Q7p) # this does not put a first
eig3.remove(a)
eig3=[a]+eig3
```

Here is the promised verification that  $a$  and its conjugates really are the 3 eigenvalues of  $T_2$  on  $V_3$ plus:

```
sage: Set(eig3) == Set(T2V3plus.change_ring(Q7p).eigenvalues())
True
```

To get all 36 eigenvalues of  $T_2$  on  $W$ plus we multiply these by the 12th roots of unity:

```
eig12 = [a*zeta12^j for j in range(12)]
eig36 = sum([[Q84(ai)*zeta12^j for j in range(12)] for ai in eig3], [])
eig9 = sum([[eig36[12*i+4*j] for i in range(3)] for j in range(3)], [])
sage: all([T2Wplus.charpoly()(l)==0 for l in eig36])
True
```

Here

$$\mathbf{eig12} = [-\zeta_{84}^{22} + \zeta_{84}^8 + \zeta_{84}^6 - 1, \zeta_{84}^{13} - \zeta_{84}^7 + \zeta_{84}, \zeta_{84}^{20} - \zeta_{84}^{14} + \zeta_{84}^8, \zeta_{84}^{23} - \zeta_{84}^{17} + \zeta_{84}^{13} + \zeta_{84}^{11} - \zeta_{84}^7 - \zeta_{84}^5 + \zeta_{84}, \zeta_{84}^{22} + \zeta_{84}^2]$$

are the eigenvalues of  $T_2$  on the 12-dimensional space spanned by the newform with  $a_2 = a$  and its twists; this 12-dimensional space is an irreducible  $\mathrm{PSL}(2, 13)$ -module over  $\mathbb{Q}(\zeta_7^+)$ . The longer list `eig36` includes all Galois conjugates over  $\mathbb{Q}$ , and is the list of all 36 eigenvalues of  $T_2$  on  $W$ plus. Lastly, `eig9` is a list of the  $T_2$ -eigenvalues on the space  $V_3$  and its Galois conjugates.

Now for the eigenvectors. We compute the first three  $T_2$ -eigenvectors with respect to the basis of  $V_3$ plus, and check that their eigenvalues are the elements of `eig3` in the correct order.

```
vec3 = [(T2V3plus-e).kernel().basis()[0] for e in eig3]
sage: all([v*T2V3plus==e*v for e,v in izip(eig3,vec3)])
```

True

The list of these 3 eigenvectors is called `vec3`; each has length 3 and entries in  $\mathbb{Q}(\zeta_7^+)$ .

Next, multiplying by the basis matrix for `V3` as a subspace of  $\mathbb{Q}^{100}$  we obtain the corresponding three eigenvectors for  $T_2$ .

```
longevec3 = [e*V3plus.basis_matrix() for e in vec3]
```

```
sage: all([v*T2==ev*v for v,ev in izip(longevec3,eig3)])
```

True

The list of these 3 eigenvectors is called `longevec3`; each has length 100 and entries in  $\mathbb{Q}(\zeta_7^+)$ .

To compute the remaining eigenvectors which are an eigenbasis for the 36-dimensional space `Wplus`, we apply the twisting operator  $R_\varepsilon$  to these; this is quicker than calling `kernel()` many more times, and also ensures that the conjugate eigenvectors are coherently scaled.

To do this we first need to define the characters modulo 13. The character group is generated by `eps` =  $\varepsilon$  of order 12, normalised so that  $\varepsilon(2) = \zeta_{12}$ . We also use `chi` =  $\chi = \varepsilon^4$  of order 3. We ensure that their values are in the field  $\mathbb{Q}(\zeta_{12}) \subset \mathbb{Q}(\zeta_{1092})$  as constructed earlier.

```
eps = [eps for eps in DirichletGroup(13,base_ring=Q12)
        if eps(2)==zeta12][0]
chi = eps^4
chibar = chi^2
epsbar = eps^(-1)
```

Next we compute the Gauss sum for  $\varepsilon$  and its conjugate, which lie in  $\mathbb{Q}(\zeta_{84})$ :

```
geps = sum([zeta13^i*eps(i) for i in range(13)])
gepsbar = sum([zeta13^i*epsbar(i) for i in range(13)])
```

The following vectors of scalings will be used to attach the correct weights to eigenforms. The point is that we will express  $A_4$ -invariant eigenvectors in the space of cuspidal modular symbols as linear combinations of the Hecke eigenvectors, and want to get hold of the  $q$ -expansions of the corresponding cusp forms as linear combinations of the (normalized) eigenforms; but there is not obvious way of normalizing elements of the modular symbol space. The mathematics behind this scaling has been written up separately.

```
gepsvec = vector([geps^i for i in range(12)])
gepsvecm = vector([(-geps)^i for i in range(12)])
```

Now we use iteration to find  $T^i$  for  $0 \leq i < 13$ , as  $100 \times 100$  matrices over  $\mathbb{Q}$ , then base-change these to  $100 \times 100$  matrices over  $\mathbb{Q}(\zeta_{12})$  so we can take linear combinations of them with coefficients which are character values.

```

Tpowers=[I]
while len(Tpowers)<13: Tpowers+=[T*Tpowers[-1]]
TpowersQ12 = [M.change_ring(Q12) for M in Tpowers]

```

Using these powers of  $T$ , we form the twisting operators:

```

Repsbar = sum([eps(i)*TpowersQ12[i] for i in range(13)])
Reps = sum([epsbar(i)*TpowersQ12[i] for i in range(13)])
Rchibar = sum([chi(i)*TpowersQ12[i] for i in range(13)])
Rchi = sum([chibar(i)*TpowersQ12[i] for i in range(13)])

```

```

sage: Conj*Reps==Reps*Conj and T*Reps==Reps*T and Conj*Rchi==Rchi*Conj and T*Rchi==Rchi*T

```

True

Note that  $T$  commutes with both  $\text{Reps}$  and  $\text{Rchi}$ , but that  $\text{Conj}$  commutes with  $\text{Rchi}$  but anticommutes with  $\text{Reps}$ . This is because  $\varepsilon(-1) = -1$  while  $\chi(-1) = +1$ .

Now we compute the 12 eigenvectors as twists of the first one, each as a list representing an elements of  $\mathbb{Q}(\zeta_{84})^{100}$ :

```

longevec12=[(longevec3[0]).change_ring(Q84)]
R=Repsbar.change_ring(Q84)
while len(longevec12)<12: longevec12+=[R*longevec12[-1]]

```

If we twist one further time we will get a multiple of the original vector, since  $R_{\varepsilon}^{12}$  is a scalar multiple of the identity.

```

sage: r = -1894464*zeta12^3 + 396825*zeta12^2 + 161460*zeta12 + 4259255

```

```

sage: R*longevec12[11]==r*longevec12[0]

```

True

```

sage: r.norm().factor()

```

$13^{24}$

We now have 12 eigenvectors in  $\mathbb{Q}(\zeta_{84})^{100}$  spanning a 12-dimensional space called  $\text{W1}$ . The 36-dimensional space  $\text{Wplus}$  we had earlier is the sum of this and its (cubic) Galois conjugates.

```

W1=longevec12[0].parent().subspace(longevec12)
Mlongevec12 = Matrix(longevec12)

```

The rows of the  $12 \times 100$  matrix  $\text{Mlongevec2}$  are the eigenvectors in  $\text{longevec12}$ , which span  $\text{W1}$ : note that  $\text{W1.basis_matrix}()$  will not be equal to this as it has been echelonised when the space  $\text{W1}$  was constructed.

$\text{W1}$  is an irreducible representation space for  $\text{PSL}(2, 13)$ , which happens to have a 1-dimensional  $A_4$ -invariant subspace. It is really defined over the cubic field  $\mathbb{Q}(\zeta_7^+)$ , but we have extended scalars to  $\mathbb{Q}(\zeta_{84})$  which contains  $\mathbb{Q}(\zeta_7^+)(\zeta_{12})$ .

On the 12-dimensional space  $\text{W1}$ , the action of  $\text{PSL}(2, 13)$  is via the images of  $S$  and  $T$ , and  $A_4$  acts as before using its generators  $A, B$ :

```

TW1 = T.transpose().change_ring(Q84).restrict(W1)
SW1 = S.transpose().change_ring(Q84).restrict(W1)
AW1 = A.transpose().change_ring(Q84).restrict(W1)
BW1 = B.transpose().change_ring(Q84).restrict(W1)
AW1d = BW1^(-1)*AW1*BW1
sigmaW1 = (1+AW1)*(1+AW1d)*(1+BW1+BW1^2)

```

```
sage: sigmaW1.rank()
```

1

```
sage: sigmaW1*(sigmaW1-12) == 0
```

True

As with `sigma` earlier, `sigmaW1` is the sum of the  $A_4$ -action matrices, and projects  $W1$  onto the 1-dimensional  $A_4$ -invariant subspace. (Strictly, `sigmaW1` is 12 times the projector.)

The  $A_4$ -invariant subspace of  $W1$  is 1-dimensional, so we pick its first basis vector and name it `Aw4_inv_W1`, then check that it really is  $A_4$ -invariant:

```
sage: sigmaW1.row_space().dimension()
```

1

```
sage: A4_inv_W1 = sigmaW1.row_space().basis()[0]
```

```
sage: all([A4_inv_W1*g == A4_inv_W1 for g in [AW1,BW1]])
```

True

The coordinates of `A4_inv_W1` are with respect to the echelon basis of  $W1$ , but we want its coordinates with respect to our original basis of Hecke eigenvectors (each the image of the previous under the twist `Repsbar`) which are the rows of `Mlongevec12`. We compute this by solving a linear system, giving a new coordinate vector of the same length, called `A4_inv_1`:

```
A4_inv_1 = Mlongevec12.solve_left(A4_inv_W1*W1.basis_matrix())
```

From earlier calculations we know that the only twists which appear here, i.e. the only nonzero entries in the vector `A4_inv_1`, are those indexed by multiples of 4, i.e. the twists by powers of  $\chi = \varepsilon^4$ :

```
sage: all([A4_inv_1[i]==0 for i in [1,2,3, 5,6,7, 9,10,11]])
```

True

We pick out the nonzero coordinates of this  $A_4$ -invariant vector, which give its coordinates with respect to the  $1, \chi, \chi^2$  twists:

```
coeffs1=[A4_inv_1[4*i] for i in range(3)]
```

We compute an automorphism of  $\mathbb{Q}(\zeta_{84})$  which fixes  $\zeta_{12}$  and acts nontrivially on  $\zeta_7^+$ . Those which fix  $\zeta_{12}$  form a group of order 6, of which 2 fix  $\zeta_7^+$ , leaving 4, with only 2 different restrictions to  $\mathbb{Q}(\zeta_7^+)$ , one the inverse of the other. Some experimentation was needed to get the 3-cycle the right way round here which turned to be with the automorphism indexed 1:

```
aut7 = [aut for aut in Q84.automorphisms()
        if aut(zeta12)==zeta12 and aut(zeta7p)!=zeta7p][1]
```

We check that our automorphism called `aut7` cycles round the basic 3  $T_2$ -eigenvalues in the right direction:

```
sage: all([aut7(eig3[i])==eig3[(i+1)%3] for i in range(3)])
True
```

Recall that `coeffs1` gives the 3 coefficients of an  $A_4$ -invariant vector in terms of the  $1, \chi, \chi^2$  twists of the original  $T_2$ -eigenvector. To get the other two  $A_4$ -invariant vectors we apply our automorphism to these:

```
coeffs2 = [aut7(c) for c in coeffs1]
coeffs3 = [aut7(c) for c in coeffs2]
coeffs = [coeffs1, coeffs2, coeffs3]
```

Each of these coefficient vectors gives the coefficients of an  $A_4$ -invariant vector with respect to vectors in the modular symbol space which are each Hecke eigenvectors, but whose relative scaling is such that the twisting operator `Repsbar` maps them round cyclically. The theory of twisting operators (see Atkin and Li) tells us that the corresponding  $A_4$ -invariant linear combinations of the normalised newforms must use as coefficients not these coefficients exactly, but these scaled by powers of the Gauss sum: this is because the twisting operators takes a normalised eigenform to another eigenform which is not normalised but scaled by a Gauss sum. We have already computed the required powers. So each of the three elements of the list `coeffs_scaled` is a list of three coefficients such that when we take these linear combinations of the newforms, we will get an  $A_4$ -invariant  $q$ -expansion. [In fact they will also need to be complex-conjugated later.]

```
coeffs_scaled=[[c*geps^(4*i) for i,c in enumerate(co)] for co in coeffs]
```

## 5 $q$ -expansions of newforms and $A_4$ -invariant cusp forms

Now we construct the  $q$ -expansion of a basis for the  $A_4$ -invariant cusp forms, starting with the  $q$ -expansion of the newforms and taking appropriate linear combinations.

The 9 relevant newforms have  $q$ -expansions which are power series in  $\mathbb{Q}(\zeta_{1092})[[q]]$ . They actually have coefficients in  $\mathbb{Q}(\zeta_{12}, \zeta_7^+) \subset \mathbb{Q}(\zeta_{84})$ , but we need to extend scalars to include  $\zeta_{13}$  so that we can take linear combinations weighted by powers of Gauss sums, so we will embed them in  $\mathbb{Q}(\zeta_{1092})[[q]]$ .

```
f = S3.q_eigenform(ps_prec, 'alpha')
g = S8.q_eigenform(ps_prec, 'beta')
```

The coefficient field  $\mathbb{Q}(f) = \mathbb{Q}(\alpha) = \mathbb{Q}(\zeta_7^+)$  is a subfield of  $\mathbb{Q}(\zeta_{1092})$ . We order the embeddings  $\mathbb{Q}(\alpha) \hookrightarrow \mathbb{Q}(\zeta_{1092})$  so that the  $i$ 'th one takes  $\alpha$  to  $\text{eig3}[i]$  for  $i = 0, 1, 2$ .

```
Kf=f.parent().base_ring()
alpha=Kf.gen()
embsKfQ84=Kf.embeddings(Q84)
emb3=[[e for e in embsKfQ84 if e(alpha)==ev][0] for ev in eig3]
sage: all([e(alpha)==ev for e, ev in izip(emb3, eig3)])
```

True

Similarly,  $\mathbb{Q}(g) = \mathbb{Q}(\beta) = \mathbb{Q}(\zeta_7^+, \zeta_3)$  is also a subfield of  $\mathbb{Q}(\zeta_{1092})$ . We order the embeddings  $\mathbb{Q}(\beta) \hookrightarrow \mathbb{Q}(\zeta_{1092})$  so that the  $i$ 'th one takes  $\beta$  to  $\text{eig9}[i+3]$  for  $0 \leq i < 6$ .

```
Kg=g.parent().base_ring()
beta=Kg.gen()
embsKgQ84=Kg.embeddings(Q84)
emb8=[[e for e in embsKgQ84 if e(beta)==ev][0] for ev in eig9[3:]]
sage: assert all([e(beta)==ev for e, ev in izip(emb8, eig9[3:])])
```

To get  $q$ -expansions for all 9 newforms in  $\mathbb{Q}(\zeta_{1092})[[q]]$ , we apply the three embeddings of  $\mathbb{Q}(\alpha)$  to the coefficients of  $f$ , and the six embeddings of  $\mathbb{Q}(\beta)$  to  $g$ . The resulting list of 9  $q$ -expansions will be called  $\text{f\_conj}$ s.

```
f_conjs = [Q1092q([Q1092(e(c)) for c in f.list()]) for e in emb3]
g_conjs = [Q1092q([Q1092(e(c)) for c in g.list()]) for e in emb8]
f_conjs = f_conjs + g_conjs
```

Now these 9  $\text{f\_conj}$ s are  $q$ -expansions of the 9 normalized newforms, in  $\mathbb{Q}(\zeta_{1092})[[q]]$ . Each  $q$ -expansion starts  $q + eq^2 + \dots$  where  $e$  is the  $T_2$ -eigenvalue:

```
sage: all([fi.list()[3]==[0,1,e] for fi,e in izip(f_conjs, eig9)])
```

True

We also verify that twisting by  $\chi$  cycles the newforms round as it should, at least for the first 20  $q$ -coefficients:

```
sage: all([gi==chi(i)*fi for i,fi,gi in izip(range(20),list(f_conjs[j]),list(f_conjs[(j+3)
True
```

We now construct a basis for the  $A_4$ -invariant cusp forms by taking suitable linear combinations of the 9 newforms. Then we will find the algebraic relation between them which gives a model for the associated modular curve.

Recall that the first  $A_4$ -invariant cusp form is a linear combination of  $f$  and its twists by the cubic character  $\chi$ . The coefficients in this linear combination have been computed above as `coeffs_scaled`, but they also need to be complex conjugated. See Corollary 3.16 in my notes for this; it is not easy to see why this complex conjugation is necessary, but it concerns the duality between modular symbols and cusp forms which is a duality over  $\mathbb{R}$  but not quite over  $\mathbb{C}$ .

```
coeffs_scaled_conj = [[conj1092(c) for c in ci] for ci in coeffs_scaled]
```

Now, at last, we can form three  $q$ -expansions giving a basis for the  $A_4$ -invariant cusp forms.

```
hs = [sum([coeffs_scaled_conj[j][i]*f_conjs[3*i+j]
for i in range(3)]) for j in range(3)]
```

These  $q$ -expansions (in `hs`) have coefficients in  $\mathbb{Q}(\zeta_{1092})$ , and in fact they lie in a subfield of  $\mathbb{Q}(\zeta_{1092})$  of degree 9, namely the composite  $\mathbb{Q}(\zeta_7^+, \zeta_{13}^{++})$ . But there is a basis which has coefficients in the smaller field  $\mathbb{Q}(\zeta_{13}^{++})$  (though not over  $\mathbb{Q}$ ) which we find by Galois theory. At the same time we make a second change of basis over  $\mathbb{Q}$  which (as it will turn out) simplifies the quartic equation for the modular curve, moving three of its rational points to  $[1 : 0 : 0]$ ,  $[0 : 1 : 0]$  and  $[0 : 0 : 1]$ .

```
MK7 = Matrix([[e^j for j in range(3)] for e in eig3])
MM = Matrix([[1,4,3], [-4,-3,1], [6,-2,5]]) * MK7^(-1)
hh = list(MM * vector(hs))
```

## 6 Finding the quartic relation giving the equation for $X_{A_4}(13)$

The three new  $q$ -expansions in `hh` still have  $\mathbb{Q}(\zeta_{1092})[[q]]$  as their parent though they do in fact lie in  $\mathbb{Q}(\zeta_{13}^{++})$ ; we use the embedding  $\mathbb{Q}(\zeta_{13}) \hookrightarrow \mathbb{Q}(\zeta_{1092})$  to redefine them as elements of  $\mathbb{Q}(\zeta_{13})[[q]]$ . This gives a new triple of  $q$ -expansions called `ff` which are mathematically the same as `hh` but are in  $\mathbb{Q}(\zeta_{13})[[q]]$ .

```
A4_forms = [Q13q([eQ13Q1092.preimage(c) for c in h]) for h in hh]
```

Using these we find a quartic algebraic relation between them, by finding a linear relation between all the 15 monomials.

```
RXYZ.<X,Y,Z> = QQ[]
mons4 = ((X+Y+Z)^4).monomials()
```

Form the 15 monomial combinations of the `A4_forms` and check that there is a unique linear relation between them (using the first 30 coefficients in the  $q$ -expansions):

```
h4s = [m(A4_forms) for m in mons4]
relmat = Matrix([[list(G)[i] for i in range(30)] for G in h4s])

sage: relmat.nullity()
```

1

Now compute that relation. In fact, although we have been doing linear algebra over  $\mathbb{Q}(\zeta_{13})$ , the coefficients are in  $\mathbb{Q}$  (and even in  $\mathbb{Z}$  after scaling by a factor 4):

```
polA4 = sum([c*m for c,m in izip(relmat.kernel().basis()[0],mons4)])
polA4 = 4*polA4.change_ring(QQ)
```

We check that the polynomial relation holds to the  $q$ -adic precision used.

```
sage: polA4(A4_forms).valuation() > ps_prec
```

True

The polynomial we find is

$$4X^3Y - 3X^2Y^2 + 3XY^3 - X^3Z + 16X^2YZ - 11XY^2Z + 5Y^3Z + 3X^2Z^2 + 9XYZ^2 + Y^2Z^2 + XZ^3 + 2YZ^3.$$

Using this homogeneous quartic we construct the curve  $X_{A_4}(13)$  as a plane curve, check that it is smooth and has genus 3 (as it must, though I do not have a way of showing *a priori* that it is not hyperelliptic). Here we construct the curve over  $\mathbb{Q}(\zeta_{13})$  and not over  $\mathbb{Q}$  since we will later construct some points on it, including the cusps, and these are not rational but defined over  $\mathbb{Q}(\zeta_{13})$ .

```
XA413=Curve(polA4.change_ring(Q13))
```

We check that this plane quartic is smooth and of genus 3:

```
sage: XA413.is_smooth()
```

True

```
sage: XA413.genus()
```

3

## 7 Points on $X_{A_4}(13)$ : I

Before computing all the 7 cusps, we construct some “easy” points, including 4 rational points. Three of these four rational points have the simplest possible coordinates only because of the change of basis we used earlier:

```
sage: PtsQ = [XA413(1,0,0), XA413(0,1,0), XA413(0,0,1), XA413(1,3,-2)]
sage: PtsQ
```

$$\left[ (1:0:0), (0:1:0), (0:0:1), \left(-\frac{1}{2} : -\frac{3}{2} : 1\right) \right]$$

In fact, searching for rational points up to bound 5 finds no more points:

```
sage: [XA413(list(p)) for p in Curve(polA4).rational_points(bound=5)]
```

$$\left[ \left(-\frac{1}{2} : -\frac{3}{2} : 1\right), (0:0:1), (0:1:0), (1:0:0) \right]$$

Next, the cusp infinity is easy to compute as its coordinates are simply the leading coefficients of the three  $q$ -expansions. This gives a point of degree 3, defined over  $\mathbb{Q}(\zeta_{13}^{++})$ , and we also compute its Galois conjugates (which are also cusps):

```
pt = [f[1] for f in A4_forms]
PtsQ13 = [XA413(pt), XA413([Q13sigma(c) for c in pt]),
          XA413([Q13sigma(Q13sigma(c)) for c in pt])]
Pts = PtsQ + PtsQ13
```

So far we have 7 points, of which 4 are rational and 3 are defined over  $\mathbb{Q}(\zeta_{13})$  (in fact over  $\mathbb{Q}(\zeta_{13}^{++})$ ):

```
sage: PtsQ13[0]
```

$$\left( \frac{4}{5}\zeta_{13}^{11} + \frac{4}{5}\zeta_{13}^{10} + \frac{1}{5}\zeta_{13}^9 + \frac{1}{5}\zeta_{13}^7 + \frac{1}{5}\zeta_{13}^6 + \frac{1}{5}\zeta_{13}^4 + \frac{4}{5}\zeta_{13}^3 + \frac{4}{5}\zeta_{13}^2 - \frac{4}{5} : -\frac{7}{5}\zeta_{13}^{11} - \frac{7}{5}\zeta_{13}^{10} - \frac{3}{5}\zeta_{13}^9 - \frac{3}{5}\zeta_{13}^7 - \frac{3}{5}\zeta_{13}^6 - \frac{3}{5}\zeta_{13}^4 \right)$$

```
sage: PtsQ13[1]
```

$$\left( -\frac{3}{5}\zeta_{13}^{11} - \frac{3}{5}\zeta_{13}^{10} - \frac{4}{5}\zeta_{13}^9 - \frac{4}{5}\zeta_{13}^7 - \frac{4}{5}\zeta_{13}^6 - \frac{4}{5}\zeta_{13}^4 - \frac{3}{5}\zeta_{13}^3 - \frac{3}{5}\zeta_{13}^2 - \frac{8}{5} : \frac{4}{5}\zeta_{13}^{11} + \frac{4}{5}\zeta_{13}^{10} + \frac{7}{5}\zeta_{13}^9 + \frac{7}{5}\zeta_{13}^7 + \frac{7}{5}\zeta_{13}^6 + \frac{7}{5}\zeta_{13}^4 \right)$$

```
sage: PtsQ13[2]
```

$$\left( -\frac{1}{5}\zeta_{13}^{11} - \frac{1}{5}\zeta_{13}^{10} + \frac{3}{5}\zeta_{13}^9 + \frac{3}{5}\zeta_{13}^7 + \frac{3}{5}\zeta_{13}^6 + \frac{3}{5}\zeta_{13}^4 - \frac{1}{5}\zeta_{13}^3 - \frac{1}{5}\zeta_{13}^2 - 1 : \frac{3}{5}\zeta_{13}^{11} + \frac{3}{5}\zeta_{13}^{10} - \frac{4}{5}\zeta_{13}^9 - \frac{4}{5}\zeta_{13}^7 - \frac{4}{5}\zeta_{13}^6 - \frac{4}{5}\zeta_{13}^4 \right)$$

## 8 Points on $X_{A_4}(13)$ : II cusps

We have an explicit model for the modular curve  $X_{A_4}(13)$ , defined over  $\mathbb{Q}$ , and a parametrization of it (in fact the “canonical embedding” into  $\mathbb{P}^2$ ) using the three cusp forms of weight 2, `A4_forms` =  $(f_1, f_2, f_3)$ , which can be evaluated at any point  $\tau$  in the upper half-plane to give a point  $\alpha(\tau) = [f_1(\tau) : f_2(\tau) : f_3(\tau)] \in X_{A_4}(13)(\mathbb{C})$ . The image of the upper half-plane under this map  $\alpha$  is an open subset of  $X_{A_4}(13)$ , omitting the cusps. The image of the cusp  $\infty$  is easy to determine, since  $q$  is a local parameter there and the three  $q$ -expansions  $f_i$  are expansions of the coordinate functions  $X, Y, Z$  of our model in term of this parameter. Bearing in mind that the  $f_i$  are cusp forms and so start  $q + a_2^{(i)}q^2 \dots$  we see that  $\alpha(\infty) = [a_2^{(1)} : a_2^{(2)} : a_2^{(3)}]$  as evaluated above.

What about the other cusps? These have the form  $c = g(\infty)$  for  $g \in \text{PSL}(2, \mathbb{Z})$ , so

$$\begin{aligned} \alpha(c) &= [f_1(g(\infty)) : f_2(g(\infty)) : f_3(g(\infty))] \\ &= [(f_1|g)(\infty) : (f_2|g)(\infty) : (f_3|g)(\infty)] \\ &= [(f_1|g)[1] : (f_2|g)[1] : (f_3|g)[1]] \end{aligned}$$

where the notation  $f[1]$  means the coefficient of  $q^1$  in a  $q$ -expansion.

The cusp forms  $f_i|g$  which appear in this formula are in the 50-dimensional space of cusp forms of weight 2 for  $G$ , and even in the 36-dimensional subspace dual to the modular symbol space `Wplus`, but do not lie in the 9-dimensional subspace (spanned by `f_conjs`) we used to find the equation. This is why we constructed `Wplus`. If we can express each  $f_i|g$  explicitly as a linear combination of newforms then, since newforms are by definition normalized, we can extract the coefficient of  $q^1$  in their expansion simply by adding the coefficients in the linear combination, without needing to know all the newforms’  $q$ -expansions at all.

We now define a function to carry this plan out. By reverting from the basis  $(f_1, f_2, f_3)$  to the first basis we found for the  $A_4$ -invariants, we are able to replace one 36-dimensional computation by three 12-dimensional ones, which are conjugate over  $\mathbb{Q}(\zeta_7^{\pm})$  so in fact do a single 12-dimensional computation followed by Galois conjugation. As before, we do most of the work in the modular symbol space. Suppose that `gam` is the  $12 \times 12$  matrix giving the action of an element  $g \in \text{PSL}(2, \mathbb{Z})$  on the 12-dimensional modular symbol space `W1`, viewed as a subspace of  $\mathbb{Q}(\zeta_{84})^{100}$ . For example, the generators  $S$  and  $T$  of  $\text{PSL}(2, \mathbb{Z})$  act via the matrices `SW1` and `TW1`. More generally, we construct such `gam` by writing  $g$  as a word in  $S, T$  and setting `gam` to be the same word in `SW1, TW1`.

Given the  $12 \times 12$  matrix `gam` we proceed as follows:

1. Multiply `gam` by the  $A_4$ -invariant vector `A4_inv_W1` in `W1`, and then by the basis matrix of `W1` to get a vector in  $\mathbb{Q}(\zeta_{84})^{100}$ , then express this as a linear combination of the eigenbasis for `W1`.
2. Apply the order 3 Galois automorphism to the resulting vector (denoted `v1` in the code below, and of length 12) get two more vectors (denoted `v2`

and  $v_3$ ); these three vectors are a basis for the image of the  $A_4$ -invariant vectors under  $\text{gam}$ .

3. Change basis (using matrix  $\text{MM}$ ) and scale by Gauss sums and complex conjugation to get the coordinates of the images of  $f_1, f_2, f_3$  under  $g$  with respect to the newform basis, and add up these coordinates to obtain the  $q^1$ -coefficient. (In the code below this is done using an inner product.)
4. This gives a vector of three homogeneous coordinates, in  $\mathbb{Q}(\zeta_{84})$ , of the desired point; finally divide by the last nonzero coordinate and pull back to  $\mathbb{Q}(\zeta_{13})$  to get a point in  $X_{A_4}(13)(\mathbb{Q}(\zeta_{13}))$ .

This is achieved by the following Sage function:

```
def get_cusp(gam): # returns coords of cusp gam(infinity)
    v1 = Mlongevec12.solve_left(A4_inv_W1*gam*W1.basis_matrix())
    v2 = [aut7(c) for c in v1]
    v3 = [aut7(c) for c in v2]
    p2 = list(MM*Matrix([v1,v2,v3])*gepsvecm)
    p2 = [conj1092(c) for c in p2] # complex conjugation
    p2 = [c/p2[2] for c in p2] # normalize so last coordinate is 1
    assert polA4(p2)==0
    p2 = [eQ13Q1092.preimage(c) for c in p2] # pull back to Q13
    assert polA4(p2)==0
    return p2
```

For example, the cusp  $\infty$  itself maps to

$$\alpha(\infty) = \left( \frac{4}{5}\zeta_{13}^{11} + \frac{4}{5}\zeta_{13}^{10} + \frac{1}{5}\zeta_{13}^9 + \frac{1}{5}\zeta_{13}^7 + \frac{1}{5}\zeta_{13}^6 + \frac{1}{5}\zeta_{13}^4 + \frac{4}{5}\zeta_{13}^3 + \frac{4}{5}\zeta_{13}^2 - \frac{4}{5} : -\frac{7}{5}\zeta_{13}^{11} - \frac{7}{5}\zeta_{13}^{10} - \frac{3}{5}\zeta_{13}^9 - \frac{3}{5}\zeta_{13}^7 - \frac{3}{5}\zeta_{13}^6 \right)$$

All but one of the 7 cusps for  $G$  are represented by integers in  $\mathbb{P}^1(\mathbb{Q})$ : one can check that modulo  $G$  we have

$$0 \sim \infty, \quad 1 \sim 5 \sim 8 \sim 12, \quad 2 \sim 7, \quad 3 \sim 4, \quad 6 \sim 11, \quad 9 \sim 10;$$

we represent these as  $g(\infty)$  where  $g = T^j S$ . The last cusp is  $7/6 = g(\infty)$  for  $g = TST^{-6}S$ . (The computation of cusp equivalences was done separately.) Here is a function for the integral cusps:

```
def get_integral_cusp(j):
    return get_cusp(TW1^j*SW1)
```

which we apply to get 6 of the 7 cusps:

```
XA413_cusps = [XA413(get_integral_cusp(j)) for j in [0,1,2,9,6,3]]
```

For the last cusp we have

```
gam = TW1*SW1*TW1^(-6)*SW1
P = XA413(get_cusp(gam))
XA413_cusps.insert(2,P)
```

So we now have all 7 as points in  $X_{A_4}(13)(\mathbb{Q}(\zeta_{13}))$ :

sage: XA413\_cusps[0]

$$\left(\frac{4}{5}\zeta_{13}^{11} + \frac{4}{5}\zeta_{13}^{10} + \frac{1}{5}\zeta_{13}^9 + \frac{1}{5}\zeta_{13}^7 + \frac{1}{5}\zeta_{13}^6 + \frac{1}{5}\zeta_{13}^4 + \frac{4}{5}\zeta_{13}^3 + \frac{4}{5}\zeta_{13}^2 - \frac{4}{5} : -\frac{7}{5}\zeta_{13}^{11} - \frac{7}{5}\zeta_{13}^{10} - \frac{3}{5}\zeta_{13}^9 - \frac{3}{5}\zeta_{13}^7 - \frac{3}{5}\zeta_{13}^6 - \frac{3}{5}\zeta_{13}^4\right)$$

sage: XA413\_cusps[1]

$$\left(-\frac{3}{5}\zeta_{13}^{11} - \frac{3}{5}\zeta_{13}^{10} - \frac{4}{5}\zeta_{13}^9 - \frac{4}{5}\zeta_{13}^7 - \frac{4}{5}\zeta_{13}^6 - \frac{4}{5}\zeta_{13}^4 - \frac{3}{5}\zeta_{13}^3 - \frac{3}{5}\zeta_{13}^2 - \frac{8}{5} : \frac{4}{5}\zeta_{13}^{11} + \frac{4}{5}\zeta_{13}^{10} + \frac{7}{5}\zeta_{13}^9 + \frac{7}{5}\zeta_{13}^7 + \frac{7}{5}\zeta_{13}^6 + \frac{7}{5}\zeta_{13}^4\right)$$

sage: XA413\_cusps[2]

$$\left(-\frac{1}{5}\zeta_{13}^{11} - \frac{1}{5}\zeta_{13}^{10} + \frac{3}{5}\zeta_{13}^9 + \frac{3}{5}\zeta_{13}^7 + \frac{3}{5}\zeta_{13}^6 + \frac{3}{5}\zeta_{13}^4 - \frac{1}{5}\zeta_{13}^3 - \frac{1}{5}\zeta_{13}^2 - 1 : \frac{3}{5}\zeta_{13}^{11} + \frac{3}{5}\zeta_{13}^{10} - \frac{4}{5}\zeta_{13}^9 - \frac{4}{5}\zeta_{13}^7 - \frac{4}{5}\zeta_{13}^6 - \frac{4}{5}\zeta_{13}^4\right)$$

sage: XA413\_cusps[3]

$$\left(-\frac{1}{3}\zeta_{13}^{11} - \frac{1}{3}\zeta_{13}^9 - \frac{1}{3}\zeta_{13}^8 - \frac{1}{3}\zeta_{13}^7 + \frac{1}{3}\zeta_{13}^6 + \frac{1}{3}\zeta_{13}^5 - \frac{1}{3}\zeta_{13}^3 + \frac{1}{3}\zeta_{13}^2 - \frac{1}{3}\zeta_{13} - 1 : \frac{1}{9}\zeta_{13}^{11} - \frac{5}{9}\zeta_{13}^9 + \frac{1}{9}\zeta_{13}^8 + \frac{1}{9}\zeta_{13}^7 + \frac{2}{9}\zeta_{13}^6\right)$$

sage: XA413\_cusps[4]

$$\left(\frac{2}{3}\zeta_{13}^9 + \frac{1}{3}\zeta_{13}^6 + \frac{1}{3}\zeta_{13}^5 + \frac{2}{3}\zeta_{13}^3 + \frac{1}{3}\zeta_{13}^2 + \frac{2}{3}\zeta_{13} - \frac{2}{3} : -\frac{2}{3}\zeta_{13}^{11} + \frac{1}{9}\zeta_{13}^9 - \frac{2}{3}\zeta_{13}^8 - \frac{2}{3}\zeta_{13}^7 - \frac{1}{9}\zeta_{13}^6 - \frac{1}{9}\zeta_{13}^5 + \frac{1}{9}\zeta_{13}^3 - \frac{1}{9}\zeta_{13}^2\right)$$

sage: XA413\_cusps[5]

$$\left(\frac{2}{3}\zeta_{13}^{11} + \frac{1}{3}\zeta_{13}^9 + \frac{2}{3}\zeta_{13}^8 + \frac{2}{3}\zeta_{13}^7 + \frac{1}{3}\zeta_{13}^3 + \frac{1}{3}\zeta_{13} - \frac{2}{3} : \frac{7}{9}\zeta_{13}^{11} + \frac{5}{9}\zeta_{13}^9 + \frac{7}{9}\zeta_{13}^8 + \frac{7}{9}\zeta_{13}^7 + \frac{2}{3}\zeta_{13}^6 + \frac{2}{3}\zeta_{13}^5 + \frac{5}{9}\zeta_{13}^3 + \frac{2}{3}\zeta_{13}^2\right)$$

sage: XA413\_cusps[6]

$$\left(-\frac{1}{3}\zeta_{13}^{11} - \frac{2}{3}\zeta_{13}^9 - \frac{1}{3}\zeta_{13}^8 - \frac{1}{3}\zeta_{13}^7 - \frac{2}{3}\zeta_{13}^6 - \frac{2}{3}\zeta_{13}^5 - \frac{2}{3}\zeta_{13}^3 - \frac{2}{3}\zeta_{13}^2 - \frac{2}{3}\zeta_{13} - \frac{4}{3} : -\frac{2}{9}\zeta_{13}^{11} - \frac{1}{9}\zeta_{13}^9 - \frac{2}{9}\zeta_{13}^8 - \frac{2}{9}\zeta_{13}^7 - \frac{7}{9}\zeta_{13}^6\right)$$

Their degrees are

sage: [max([co.minpoly().degree() for co in list(c)]) for c in XA413\_cusps]

[3, 3, 3, 4, 4, 4, 4]

## 9 The $j$ -map $X_{A_4}(13) \longrightarrow X(1)$

We now find an expression for the rational map  $j$  of degree 91 from  $X_{A_4}(13)$  to the  $j$ -line  $X(1)$ .

The poles of  $j$  are at the 7 cusps which we have computed exactly, each with multiplicity 13. The zeroes of  $j$  are harder to pin down. One approach, as used by Burcu Baran for  $X_{\text{sp}}(13)$  and  $X_{\text{ns}}(13)$ , is to use the parametrisation of  $X_{A_4}(13)$  by modular functions on the upper half-plane. Write  $X, Y, Z$  for the three cusp forms denoted `A4_forms` above. Then the parametrizing map

$$\varphi : \mathcal{H} \rightarrow X_{A_4}(13)(\mathbb{C})$$

is given by  $\tau \mapsto [X(q) : Y(q) : Z(q)]$  with  $q = \exp(2\pi i\tau)$ . We can extend this map to the cusps as indicated in the previous section. Now the zeroes of  $j$  are the points  $\varphi(\tau)$  such that  $j(\tau) = 0$ : there are 91 of these, counting multiplicities (in fact 29 have multiplicity 3 and 4 have multiplicity 1), coming from the elliptic points of order 3 on the upper half-plane  $\mathcal{H}$ .

Baran's approach is to compute  $\varphi(\tau)$  numerically from the  $q$ -expansions for 91 (or in fact  $29+4 = 33$ ) elliptic points  $\tau$  and hence recognise these as algebraic points. If successful, then one has the complete divisor of  $j$  as a rational function on the curve and can use Riemann-Roch to find  $j$ .

Instead we proceed as follows. First we find a polynomial in  $X, Y, Z$  passing through the 7 cusps. There are no quadratics through these points:

```
sage: mons2 = ((X+Y+Z)^2).monomials()
sage: matrix([[m(list(c)) for c in XA413_cusps] for m in mons2]).nullity()
0
```

but there are cubics:

```
sage: mons3 = ((X+Y+Z)^3).monomials()
sage: ker = matrix([[m(list(c)) for c in XA413_cusps] for m in mons3]).left_kernel()
sage: ker.dimension()
3
```

We find an LLL-reduced basis for the integral cubics in this 3-dimensional space:

```
M = ker.basis_matrix()
M = (M*M.denominator()).change_ring(ZZ)
Sm,U,V = M.smith_form()
M = (Sm.submatrix(ncols=3)^(-1)*U*M).change_ring(ZZ)
M = (M*M.transpose()).LLL_gram().transpose() * M
cubs = [sum([c*m for c,m in izip(r,mons3)]) for r in M.rows()]
```

This gives the following cubics:

```
sage: cubs[0]
```

$$-7X^3 + X^2Y - 18X^2Z + 6XYZ - 2Y^2Z - 17XZ^2 + YZ^2 - 3Z^3$$

```
sage: cubs[1]
```

$$7X^3 + 16XY^2 + 3Y^3 + 15X^2Z - 18XYZ + 21Y^2Z - 7XZ^2 + 6YZ^2 - 3Z^3$$

```
sage: cubs[2]
```

$$5X^3 - 19X^2Y - 6XY^2 + 9Y^3 + X^2Z - 23XYZ - 16Y^2Z + 8XZ^2 - 22YZ^2 + 3Z^3$$

We do not use the first two of these as they pass through some of the rational points we know on the curve, which will cause problems later when we try to evaluate  $j$  on these points:

```
sage: cub = cubs[0]
```

```
sage: [cub(list(p)) for p in PtsQ]
```

$$[-7, 0, -3, 0]$$

Hence we use a cubic which does not have this issue

```
sage: cub = cubs[2]
```

```
sage: [cub(list(p)) for p in PtsQ]
```

$$\left[5, 9, 3, -\frac{305}{8}\right]$$

Now we convert the  $q$ -expansions of the three  $A_4$ -invariant cusp forms to lie in  $\mathbb{Q}(\zeta_{13}^{++})[[q]]$ ; at the same time we divide each by  $q$  (otherwise all the power series exponents later will be unnecessarily shifted by 39).

```
ffq = [ Q13ppq([eQ13ppQ13.preimage(c) for c in list(f)[1:]]).add_bigoh(ps_prec)
        for f in A4_forms]
xq,yq,zq = ffq
```

The denominator of  $j$  may be taken to be the 13th power of the cubic through the cusps:

$$\text{denj13} = \text{cub}(\text{ffq})^{13}$$

For  $j$  itself we must evaluate the standard  $q$ -expansion for the  $j$ -function at  $q^{13}$ :

```
jq = j_invariant_qexp(20, Q13pp)
jq13 = jq(Q13ppq.gen()^13)
```

Now the numerator of the rational function is a homogeneous polynomial of degree 39 whose coefficients we must determine so that when evaluated at the  $q$ -expansions of  $X, Y, Z$  equals  $j(q^{13})$  times the denominator:

```
numjq39 = jq13*denj13
```

We set up a system of linear equations to solve for the unknown coefficients. We do not need to use all monomials of degree 39 since the curve equation can be used to reduce the numerator polynomial.

```
sage: mons39 = ((X+Y+Z)^39).monomials()
```

```
sage: len(mons39)
```

820

```
sage: mons39r = [m for m in mons39 if m.degrees()[0]<3 or m.degrees()[1]==0]
```

```
sage: len(mons39r)
```

154

So we need at least 154 coefficients of the  $q$ -expansions. For efficiency, instead of simply evaluating all the monomials at  $X, Y, Z$  we first find all necessary powers of each variable and then combine these.

```
xpowers = [xq.parent()(1)]
```

```
ypowers = [yq.parent()(1)]
```

```
zpowers = [zq.parent()(1)]
```

```
while len(xpowers)<40:
```

```
    xpowers += [xq*xpowers[-1]]
```

```
    ypowers += [yq*ypowers[-1]]
```

```
    zpowers += [zq*zpowers[-1]]
```

```
mons39q = [xpowers[m.degrees()[0]]*ypowers[m.degrees()[1]]*zpowers[m.degrees()[2]] for m in mons39r]
```

We extract the array of the relevant coefficients; it is enough to look at the coefficients of  $q^n$  for  $n < 160$ . Significantly, since we know that the solution will be 1-dimensional and with coordinates in  $\mathbb{Q}$  we can save a lot of time by reducing to linear algebra over  $\mathbb{Q}$ :

```
arr = [ [mq[i] for i in range(160)] for mq in mons39q ] + \
```

```
    [[-numjq39[i] for i in range(160)]]
```

```
relmatQ = Matrix([ flatten([list(aij) for aij in ai]) for ai in arr ])
```

```
ker = relmatQ.left_kernel()
```

If all is well the dimension of the solution space should be 1:

```
sage: ker.dimension()
```

1

We extract the coefficients from the coordinates of the solution vector:

```
b = ker.basis()[0]
```

```
b *= b.denominator()
```

```
d = b[-1]
```

and form the numerator and denominator of the rational function we have been seeking:

```
jnum = sum([bi*m for bi,m in zip(list(b)[: -1],mons39r)])
jden = d*cub^13
```

The images of the rational points on  $X_{A_4}(13)$  give rational  $j$ -invariants of elliptic curves whose projective mod-13 Galois representation is contained in  $S_4$  (and in  $A_4$  after base change to  $\mathbb{Q}(\sqrt{13})$ ):

```
sage: [(jnum(list(p))/jden(list(p))) for p in PtsQ]
[0,  $\frac{11225615440}{1594323}$ ,  $-\frac{160855552000}{1594323}$ ,  $\frac{90616364985637924505590372621162077487104}{197650497353702094308570556640625}$ ]
```

## 10 The Split Cartan case: $X_s(13)$

This is the simplest of the three cases, since the space of cusp forms invariant under the split Cartan normaliser is spanned by 3 conjugate newforms with trivial character. We choose the split Cartan subgroup to be the subgroup of diagonal matrices: then a cusp form is invariant under the split Cartan if and only if it has trivial character, and is also invariant under the normalizer of the split Cartan if it has eigenvalue +1 for the Atkin-Lehner involution. The space of such forms is 3-dimensional and is the space spanned by the first three of the  $q$ -expansions denoted `f_conjs` above.

### 10.1 An equation for the curve

We make a change of basis here so that the equation we obtain agrees with that obtained by Burcu Baran.

```
M1 = Matrix(QQ,3,3,[-1, 1, -3, -1, 0, -1, 0, 0, 1])
SC_forms = M1 * MK7^(-1) * vector(f_conjs[:3])
SC_forms = [QQq(list(gi)).add_bigoh(ps_prec) for gi in SC_forms]
```

We find a quartic relation between these just as before; the computation is simpler since these  $q$ -expansions have rational coefficients.

```
g4s=[m([f.add_bigoh(40) for f in SC_forms]) for m in mons4]
relmat = Matrix([[list(G)[i] for i in range(30)] for G in g4s])
```

We find the polynomial (changing its sign so that `polSC` is exactly the same as Burcu's defining polynomial):

```
sage: relmat.nullity()
```

1

```
sage: polSC = -sum([c*m for c,m in zip(relmat.kernel().basis()[0],mons4)])
```

```

sage: polSC(SC_forms).valuation() > ps_prec
True

sage: polSC
-X^3Y+2X^2Y^2-XY^3-X^3Z+X^2YZ+XY^2Z-2XYZ^2+2Y^2Z^2+XZ^3-3YZ^3

```

Now we construct the curve (over  $\mathbb{Q}(\zeta_{13})$  to accommodate the cusps) and check that it is smooth and of genus 3:

```

sage: XSC13 = Curve(polSC.change_ring(Q13))

sage: XSC13.is_smooth()
True

sage: XSC13.genus()
3

```

## 10.2 Cusps and rational points

The cusps are computed as before.

```

SC_inv_W1 = vector(W1.coordinates(longevec12[0]))
def get_SC_cusp(gam): # returns coords of cusp gam(infinity)
    v1 = Mlongevec12.solve_left(SC_inv_W1*gam*W1.basis_matrix())
    v2 = [aut7(c) for c in v1]
    v3 = [aut7(c) for c in v2]
    p2 = list(M1*MK7^(-1)*Matrix([v1,v2,v3])*gepsvecm)
    p2 = [conj1092(c) for c in p2] # complex conjugation
    if p2[2]!=0: # normalize so last coordinate is 1
        p2 = [c/p2[2] for c in p2]
    else:
        if p2[1]!=0:
            p2 = [c/p2[1] for c in p2]
        else:
            p2 = [c/p2[0] for c in p2]
    assert polSC(p2)==0
    p2 = [eQ13Q1092.preimage(c) for c in p2] # pull back to Q13
    assert polSC(p2)==0
    return p2

def get_integral_SC_cusp(j):
    return get_SC_cusp(TW1^j*SW1)

XSC13_cusps = [XSC13(get_integral_SC_cusp(j)) for j in range(7)]

```

This really does find the 7 cusps, since the integers  $\{0, 1, 2, 3, 4, 5, 6\}$  represent the 7 cusps, each of width 13.

A quick search find a few rational points:

```
sage: XSC13Q = [XSC13(list(P)) for P in Curve(polSC).rational_points(bound=5)]
```

```
sage: XSC13Q
```

$$\left[ (-1 : 0 : 1), (0 : 0 : 1), (0 : 1 : 0), \left( 0 : \frac{3}{2} : 1 \right), (1 : 0 : 0), (1 : 0 : 1), (1 : 1 : 0) \right]$$

Only one cusp is rational, the others are conjugate over  $\mathbb{Q}(\zeta_{13}^+)$ :

```
sage: [P for P in XSC13_cusps if P in XSC13Q]
```

$$[(1 : 1 : 0)]$$

```
sage: XSC13_cusps[:2]
```

$$[(1 : 1 : 0), (-\zeta_{13}^{11} - \zeta_{13}^{10} - \zeta_{13}^7 - \zeta_{13}^6 - \zeta_{13}^3 - \zeta_{13}^2 : -\zeta_{13}^{10} - \zeta_{13}^9 - \zeta_{13}^8 - \zeta_{13}^7 - \zeta_{13}^6 - \zeta_{13}^5 - \zeta_{13}^4 - \zeta_{13}^3 : 1)]$$

```
sage: [max([co.minpoly().degree() for co in list(c)]) for c in XSC13_cusps]
```

$$[1, 6, 6, 6, 6, 6, 6]$$

### 10.3 Map to the $j$ -line

Now we find the rational function giving the map to the  $j$ -line. For the denominator, we check that there are no quadratics through the seven cusps:

```
sage: matrix([[m(list(c)) for c in XSC13_cusps] for m in mons2]).nullity() == 0
```

True

So we find the cubics, which again form a 3-dimensional space:

```
sage: ker = matrix([[m(list(c)) for c in XSC13_cusps] for m in mons3]).left_kernel()
```

```
sage: ker.dimension()
```

3

We clear denominators, saturate and LLL-reduce:

```
M = ker.basis_matrix()
M = (M*M.denominator()).change_ring(ZZ)
Sm,U,V = M.smith_form()
M = (Sm.submatrix(ncols=3)^(-1)*U*M).change_ring(ZZ)
M = (M*M.transpose()).LLL_gram().transpose() * M
cubs = [sum([c*m for c,m in izip(r,mons3)]) for r in M.rows()]
```

There is a rational cusp, and we will want to choose a cubic for the denominator which does not pass through any of the other rational points:

```
XSC13Q_noncusp = [P for P in XSC13Q if not P in XSC13_cusps]
sage: cubs[0], [cubs[0](list(p)) for p in XSC13Q_noncusp]
( $-X^2Y + XY^2 + XYZ - Y^2Z - 2XZ^2 + 2YZ^2 - Z^3$ ,  $\left[1, -1, 0, -\frac{1}{4}, 0, -3\right]$ )
sage: cubs[1], [cubs[1](list(p)) for p in XSC13Q_noncusp]
( $-X^3 - X^2Y + 2XY^2 + 3X^2Z - 2XYZ - Y^2Z + YZ^2 - Z^3$ ,  $\left[3, -1, 0, -\frac{7}{4}, -1, 1\right]$ )
sage: cubs[2], [cubs[2](list(p)) for p in XSC13Q_noncusp]
( $2X^2Y - 3XY^2 + Y^3 + 2X^2Z + 2XYZ - 3Y^2Z + XZ^2 + YZ^2$ ,  $\left[1, 0, 1, -\frac{15}{8}, 0, 3\right]$ )
sage: cub=cubs[1]+cubs[2]
sage: all([cub(list(p))!=0 for p in XSC13Q_noncusp])
True
sage: all([cub(list(p))==0 for p in XSC13_cusps])
True
```

To solve for the numerator we first shift the  $q$ -expansions (dividing by  $q$ ), evaluate our cubic at the resulting point and multiply by  $j(q^{13})$ :

```
ffq = [f.shift(-1) for f in SC_forms]
denj = cub(ffq)
denj13 = denj^13
jq = j_invariant_qexp(20)
q = jq.parent().gen()
jq13 = jq(q^13)
numjq39 = jq13*denj13
```

We compute an independent set of monomials of degree 39 in the  $q$ -expansions:

```
xq,yq,zq = ffq
xpowers = [xq.parent()(1)]
ypowers = [yq.parent()(1)]
zpowers = [zq.parent()(1)]
while len(xpowers)<40:
    xpowers += [xq*xpowers[-1]]
    ypowers += [yq*ypowers[-1]]
    zpowers += [zq*zpowers[-1]]

mons39r = [m for m in mons39 if m.degrees()[0]<2 or m.degrees()[1]<2]
mons39q = [xpowers[m.degrees()[0]]*ypowers[m.degrees()[1]]*zpowers[m.degrees()[2]] for m in mons39r]
```

Extract the coefficients and form the matrix whose kernel gives the coefficients of the solution:

```
relmatQ = Matrix([[mq[i] for i in range(190)] for mq in mons39q])
sol = relmatQ.solve_left(vector([numjq39[i] for i in range(190)]))
```

Using these coefficients we form the numerator and denominator as polynomials in  $\mathbb{Q}[X, Y, Z]$ :

```
c0 = sol.denominator()
c = list(c0*sol)
jnum = sum([ci*m for ci,m in zip(c,mons39r)])
jden = c0*cub^13
```

We do not display the rational function since it is huge, but we do evaluate it at some points on the curve.

#### 10.4 $j$ -invariants of rational points

Now we evaluate the map at the rational points (excluding the cusp):

```
sage: jlist = [QQ(jnum(list(p))/jden(list(p))) for p in XSC13Q_noncusp]
```

```
sage: jlist
```

```
[287496, -12288000, 54000, 0, -884736000, 1728]
```

It appears that these  $j$ -invariants are all CM, which we check:

```
sage: [j for j in jlist if not j in cm_j_invariants(QQ)]
```

```
[]
```

Finally we check that the corresponding orders agree with Burcu Baran's Table 1.1:

```
sage: CMQ = cm_j_invariants_and_orders(QQ)
```

```
sage: [(P,d*f^2) for P,jj in izip(XSC13Q_noncusp,jlist) for (d,f,j) in CMQ if j==jj]
```

```
[((-1 : 0 : 1), -16), ((0 : 0 : 1), -27), ((0 : 1 : 0), -12), ((0 : 3/2 : 1), -3), ((1 : 0 : 0), -43), ((1 : 0 : 1), -4)]
```

## 11 The Nonsplit Cartan case: $X_{ns}(13)$

The space of cusp forms invariant under the split Cartan normaliser is a 3-dimensional subspace of the 36-dimensional space of cusp forms spanned by newforms: `f_conjs` and all 12 twists of each.

We choose the nonsplit Cartan subgroup as follows.

```
B=A
A=T*S*T^(-1)*S*T*S*T^(-5)*S*T^(-1)
```

Recall that these are  $100 \times 100$  matrices giving the action of  $\mathrm{PSL}(2, 13)$  on the full modular symbol space. Their restrictions to the irreducible 12-dimensional space defined over the cubic field  $\mathbb{Q}(\zeta_{13}^{++})$  are

```
A2W1=TW1*SW1*TW1^(-1)*SW1*TW1*SW1*TW1^(-5)*SW1*TW1^(-1)
B2W1=AW1
```

which we check satisfy the defining relations for the nonsplit Cartan normaliser which is isomorphic to the dihedral group of order 14:

```
sage: (A2W1^7)==1 and (B2W1^2)==1 and (B2W1*A2W1)^2==1
True
```

We construct the projector onto the invariant subspace:

```
sage: sigmaW1 = (1+A2W1+A2W1^2+A2W1^3+A2W1^4+A2W1^5+A2W1^6)*(1+B2W1)
sage: sigmaW1.rank()==1 and sigmaW1*(sigmaW1-14)==0
True
```

Check that the invariant subspace is 1-dimensional and extract a basis vector:

```
sage: sigmaW1.row_space().dimension()
1
sage: NS_inv_W1 = sigmaW1.row_space().basis()[0]
sage: [NS_inv_W1*g == NS_inv_W1 for g in [A2W1,B2W1]]
[True, True]
```

The coordinates of `NS_inv_W1` are with respect to the echelon basis of `W1`, but we need the coordinates with respect to the eigenvector basis:

```
v = Mlongevec12.solve_left(NS_inv_W1*W1.basis_matrix())
```

In fact only the even twists occur here:

```
sage: all([(v[i]==0)==(i%2==1) for i in range(12)])
True
```

## 11.1 $q$ -expansions

We find the  $q$ -expansions of all 12 twists of the first newform:

```
f12_conjs = [Q1092q([(eps^j)(n)*(an)
                    for n,an in enumerate(list(f_conjs[0]))]).add_bigoh(ps_prec)
              for j in range(12)]
```

Using the coefficient vector  $v$  we form the  $q$ -expansion of a cusp form invariant under the nonsplit Cartan normalizer. This has been constructed with coefficients in  $\mathbb{Q}(\zeta_{1092})$  but in fact has coefficients in  $\mathbb{Q}(\zeta_{91})$ , so we pull it back to  $\mathbb{Q}(\zeta_{91})[[q]]$ , and then form the three Galois conjugates:

```
h0 = sum([conj1092(v[i]*gepsvec[i])*f12_conjs[i] for i in range(12)])
h0 = Q91q([eQ91Q1092.preimage(c) for c in list(h0)]).add_bigoh(ps_prec)
h1 = Q91q([Q91aut(c) for c in list(h0)]).add_bigoh(ps_prec)
h2 = Q91q([Q91aut(c) for c in list(h1)]).add_bigoh(ps_prec)
hh=[h0,h1,h2]
```

By taking suitable linear combinations we arrive at a basis in  $\mathbb{Q}(\zeta_{13})[[q]]$ :

```
a0=eQ91Q1092.preimage(Q1092(1/zeta7p))
a1=Q91aut(a0)
a2=Q91aut(a1)
MK7 = Matrix([[a^j for a in [a0,a1,a2]] for j in range(3)])
hh = MK7 * vector(hh)
hh = [Q13q([eQ13Q91.preimage(c)for c in h]).add_bigoh(ps_prec) for h in hh]
```

Finally we make a change of basis so that the quartic equation we find later is exactly the same as that obtained by Burcu Baran:

```
MBB = Matrix([[2,1,1],[-6,4,-3],[11,-5,2]])
NS_forms = list(MBB^(-1)*vector(hh))
```

## 11.2 Equation of the curve

We find a quartic relation between the three  $q$ -expansions in the same way as before.

```
sage: h4s=[m([h.add_bigoh(40) for h in NS_forms]) for m in mons4]
sage: relmat = Matrix([[list(G)[i] for i in range(30)] for G in h4s])
sage: relmat.nullity()
```

1

```
sage: polNS = -sum([c*m for c,m in zip(relmat.kernel().basis()[0], mons4)])
sage: polNS = polNS.change_ring(QQ)
```

```
sage: polNS == polSC
```

True

Now we construct the curve (over  $\mathbb{Q}(\zeta_{13})$  to accommodate the cusps again) and check that it is smooth and of genus 3. Although it is the same curve as before we'll construct it anyway.

```
sage: XNS13 = Curve(polNS.change_ring(Q13))
```

```
sage: XNS13.is_smooth()
```

True

```
sage: XNS13.genus()
```

3

### 11.3 Cusps and rational points

The rational points again:

```
sage: XNS13Q = [XNS13(list(p)) for p in Curve(polNS).rational_points(bound=5)]
```

```
sage: XNS13Q
```

```
[(-1 : 0 : 1), (0 : 0 : 1), (0 : 1 : 0), (0 : 3/2 : 1), (1 : 0 : 0), (1 : 0 : 1), (1 : 1 : 0)]
```

Computing the cusps is easier than before, since they are all Galois conjugates of the cusp at  $\infty$  which is easy to obtain from the  $q$ -expansions.

```
XNS13_cusps = [XNS13([(Q13aut^j)(h[1]) for h in NS_forms]) for j in range(6)]
```

The first cusp is

$$(3\zeta_{13}^{11} + \zeta_{13}^{10} + 2\zeta_{13}^9 + \zeta_{13}^8 + 2\zeta_{13}^7 + 2\zeta_{13}^6 + \zeta_{13}^5 + 2\zeta_{13}^4 + \zeta_{13}^3 + 3\zeta_{13}^2 + 2 : 2\zeta_{13}^{11} + \zeta_{13}^{10} + 2\zeta_{13}^9 + \zeta_{13}^8 + 2\zeta_{13}^7 + 2\zeta_{13}^6 + \zeta_{13}^5 + 2\zeta_{13}^4 + \zeta_{13}^3 + 3\zeta_{13}^2 + 2 : 2\zeta_{13}^{11} + \zeta_{13}^{10} + 2\zeta_{13}^9 + \zeta_{13}^8 + 2\zeta_{13}^7 + 2\zeta_{13}^6 + \zeta_{13}^5 + 2\zeta_{13}^4 + \zeta_{13}^3 + 3\zeta_{13}^2 + 2)$$

### 11.4 Map to the $j$ -line

As before there are no quadratics through the cusps:

```
sage: matrix([[m(list(c)) for c in XNS13_cusps] for m in mons2]).nullity()
```

0

so we look for cubics. As there are only 6 cusps now, the space of cubics through them has dimension  $10 - 6 = 4$ :

```
sage: ker = matrix([[m(list(c)) for c in XNS13_cusps] for m in mons3]).left_kernel()
```

```
sage: ker.dimension()
```

4

We find a small  $\mathbb{Z}$ -basis as before:

```
M = ker.basis_matrix()
M = (M*M.denominator()).change_ring(ZZ)
Sm,U,V = M.smith_form()
M = (Sm.submatrix(ncols=4)^(-1)*U*M).change_ring(ZZ)
M = (M*M.transpose()).LLL_gram().transpose() * M
cubs = [sum([c*m for c,m in izip(r,mons3)]) for r in M.rows()]
cub = cubs[0]
```

The first cubic is

$$X^3 - 3XY^2 + Y^3 + 3X^2Z - Y^2Z + 2XZ^2 - Z^3$$

which will serve as it does not pass through any of the rational points:

```
sage: [cub(list(p)) for p in PtsQ]
```

$$\left[ 1, 1, -1, -\frac{29}{8} \right]$$

```
sage: all([cub(list(p))!=0 for p in XNS13Q])
```

True

```
sage: all([cub(list(p))==0 for p in XNS13_cusps])
```

True

To ease the linear algebra it is worthwhile to convert the cusp forms to lie in  $\mathbb{Q}(\zeta_{13}^+)[[q]]$  instead of  $\mathbb{Q}(\zeta_{13})[[q]]$ . We have not used this field before so need to set this up:

```
z13p = zeta13+zeta13^12 # generates sextic subfield
Q13p.<z13p> = NumberField(z13p.minpoly(), embedding=z13p)
eQ13pQ13 = Q13p.hom([Q13(z13p)])
Q13pq.<q> = PowerSeriesRing(Q13p,ps_prec)
```

Now we do the conversion, dividing each  $q$ -expansion by  $q$  at the same time:

```
ffq = [Q13pq([eQ13pQ13.preimage(c) for c in list(f)[1:]]).add_bigoh(ps_prec-1)
        for f in NS_forms]
```

Compute the denominator, the  $q$ -expansion of  $j(q^{13})$  in the sextic field, and their product:

```

denj = cub(ffq)
denj13 = denj^13
jq = j_invariant_qexp(20, Q13p)
q = jq.parent().gen()
jq13 = jq(q^13)
numjq39 = jq13*denj13

```

Compute the degree 39 monomials:

```

xq,yq,zq = ffq
xpowers = [xq.parent()(1)]
ypowers = [yq.parent()(1)]
zpowers = [zq.parent()(1)]
while len(xpowers)<40:
    xpowers += [xq*xpowers[-1]]
    ypowers += [yq*ypowers[-1]]
    zpowers += [zq*zpowers[-1]]

```

```

mons39q = [xpowers[m.degrees()[0]]*ypowers[m.degrees()[1]]*zpowers[m.degrees()[2]] for m in range(160)]

```

Set up and solve the linear equations over  $\mathbb{Q}$ :

```

arr = [[-numjq39[i] for i in range(160)]] \
      + [[mq[i] for i in range(160)] for mq in mons39q]
relmatQ = Matrix([ flatten([list(aij) for aij in ai]) for ai in arr])
ker = relmatQ.left_kernel()

```

The solution space has dimension 1 and we extract the coefficient vector:

```

b = ker.basis()[0]
b *= b.denominator()
jnum = sum([bi*m for bi,m in zip(list(b)[1:],mons39r)])
jden = b[0]*cub^13

```

These are the numerator and denominator of the  $j$ -map, each expressed as a polynomial of degree 39 in  $\mathbb{Q}[X, Y, Z]$ .

## 11.5 $j$ -invariants of rational points

Now we evaluate the map at the rational points:

```

sage: jlist = [QQ(jnum(list(p))/jden(list(p))) for p in XNS13Q]
sage: jlist
[-3375, -147197952000, -32768, -262537412640768000, 8000, 16581375, -884736]

```

It appears that these  $j$ -invariants are all CM, which we check:

```

sage: [j for j in jlist if not j in cm_j_invariants(QQ)]

```

□

Finally we check that the corresponding orders agree with Burcu Baran's Table 1.1:

```
sage: CMQ = cm_j_invariants_and_orders(QQ)
sage: [(P,d*f^2) for P,jj in izip(XNS13Q,jlist) for (d,f,j) in CMQ if j==jj]
[((-1 : 0 : 1), -7), ((0 : 0 : 1), -67), ((0 : 1 : 0), -11), ((0 : 3/2 : 1), -163), ((1 : 0 : 0), -8), ((1 : 0 : 1), -28)]
```
